# Supplementary material for: COCA: Classifier-Oriented Calibration via Textual Prototype for Source-Free Universal Domain Adaptation
Source: arXiv:2308.10450 source file (2024-03-11)
Supplement: Supplementary file 1 [file notations.tex]

%%%%%%%%%%%%%%%%%%%% Table notations %%%%%%%%%%%%%%%%%%%%%%
\begin{table*}[t]
    \caption{\textbf{Notation Table}}
    \centering
    \resizebox{0.98\textwidth}{!}{%
        \begin{tabular}{lcl}
        \toprule
        
         & \multirow{1}{*}{Symbol} & \multirow{1}{*}{Description} \\
         \midrule

         \multirow{5}{*}{\rotatebox[origin=c]{0}{Models}} & $G^\text{img}$ & Image encoder  \\
         & $G^\text{text}$ & Text encoder \\
         & $\omega$ & Parameters of the image/text encoder \\
         & $h_\theta$ & Closed-set classifier \\
         & $h_\gamma$ & EMA teacher classifier \\
         \midrule
        
        \multirow{8}{*}{\rotatebox[origin=c]{0}{Spaces}} 
        & $C^s$ & Source/Known class set \\
        & $C^t$ & Target class set \\
        & $C$ & Common class set \\
        & $\bar{C^s}$ & Source-private class set \\
        & $\bar{C^t}$ & Target-private/unknown class set \\
        & $X$ & Target image set\\
        % & $X^\text{text}$ & Text set\\
        & $Z^\text{img}$ & Image feature set\\
        & $Z^\text{text}$ & Text feature set\\
        & $V^\text{img}$ & Image prototype set\\
        % & $\mathcal{C_I,C_J}$ & One of the $K$ clusters generated by K-means \\ 
        \midrule
        
        \multirow{11}{*}{\rotatebox[origin=c]{0}{Samples}} 
        & $x_i$ & Unlabeled target sample  \\
        & $x_i^{\mathsf{M}}$ & Unlabeled masked target sample  \\
         & \texttt{a photo of a \{CLASS\}} & Text template \\
         & $y_c$ & Ground truth label for \texttt{a photo of a \{CLASS\}}\\
         & $\hat{y}_i$ & Pseudo label for target sample $x_i$ \\
         & $z^\text{img}_i$ & Target sample feature \\
         & $z^\text{text}_c$ & Text feature for \texttt{a photo of a \{CLASS\}}\\
         & $\{v_k\}_{k=1}^K$ & Image prototype generated by K-means\\
         & $p^c$ & Image positive prototype for a known class $c$ \\
         & $\{n^c_k\}_{k=1}^{K-1}$ & Image negative prototypes for a known class $c$ \\
         & $q_i$ & Soft label generated by the teacher classifier $h_\gamma$ \\
         \midrule 
         
        \multirow{3}{*}{\rotatebox[origin=c]{0}{Measures}}  & $R_\text{IB}$ & Information Bottleneck \\
        & $I$ & Mutual Information \\
        & $U(x_i)$ & Uncertainty for target sample $x_i$ \\
        \midrule 
        
        \multirow{3}{*}{\rotatebox[origin=c]{0}{Hyperparameters}}
        & $K$ & K-means hyperparameter \\
        & $\tau$ & Threshold for distinguishing known and unknown target samples\\
        & $\mathsf{r}$ & Mask ratio \\
        \bottomrule
        \end{tabular}
        }
    \label{sup:tab:notations}
\end{table*}
%%%%%%%%%%%%%%%%%%%% Table ends %%%%%%%%%%%%%%%%%%%%%%%%%%

We summarize the notations throughout the paper in Table \ref{sup:tab:notations}. The notations are listed under five groups: models, spaces, samples, measures, and hyperparameters.
